# Supplementary material for: Evolutionary Games on Infinite Strategy Sets: Convergence to Nash Equilibria via Dissipativity
Source: arXiv:2312.08286 source file (2025-04-22)
Supplement: Supplementary file 1 [file supplementary-old.tex]

	\section{Supplementary Definitions and Results}

	\begin{definition}
		\label{def: lyapunov_function}
		Consider a game $F\colon \P(S) \to C_0(S)$ and let $v\colon \P(S) \times C_0(S) \to \M(S)$. Let $P \subseteq \P(S)$ be weakly closed. A map $V\colon \P(S) \to \Rpl$ is a \emph{global Lyapunov function for $P$ under the dynamics map $v$} if it extends to a weakly continuous Fr\'echet differentiable map $\overline{V} \colon U \to \R$ defined on a strongly open set $U\subseteq\M(S)$ containing $\P(S)$ that satisfies the following conditions:
		\begin{enumerate}
			\item $\overline{V}(\mu) = 0$ for all $\mu\in P$.
			\item $\overline{V}(\mu) > 0$ for all $\mu\in \P(S)\setminus P$.
			\item $D\overline{V}(\mu) v(\mu,F(\mu)) \le 0$ for all $\mu\in \P(S)$.
		\end{enumerate}
		If, additionally, the map $\mu \mapsto D\overline{V}(\mu) v(\mu,F(\mu))$ is weakly continuous and $D\overline{V}(\mu) v(\mu,F(\mu)) < 0$ for all $\mu\in\P(S)\setminus P$, then $V$ is a \emph{strict global Lyapunov function for $P$ under the dynamics map $v$}.
	\end{definition}

	\begin{lemma}
		\label{lem: lyapunov}
		Suppose that $S$ is compact. Consider a game $F\colon \P(S) \to C_0(S)$ and let $v\colon \P(S) \times C_0(S) \to \M(S)$. Let $P\subseteq \P(S)$ be weakly closed. If there exists a global Lyapunov function for $P$ under the dynamics map $v$, then $P$ is weakly Lyapunov stable under the dynamics map $v$.
	\end{lemma}

	\begin{proof}
		Suppose that there exists a global Lyapunov function $V\colon \P(S) \to \Rpl$ for $P$ under the dynamics map $v$, and let $\overline{V} \colon U \to \R$ be an appropriate extension as in \autoref{def: lyapunov_function}. Let $Q\subseteq \P(S)$ be relatively weakly open and contain $P$. Then $Q = \P(S)\cap O$ for some weakly open set $O\subseteq \M(S)$. Define $\partial_{\P(S)} Q \coloneqq \P(S) \cap \partial O$, where $\partial O$ is the boundary of $O$ in $\M(S)$ with respect to the weak topology. By \autoref{lem: P(S)_compact}, $\partial_{\P(S)} Q$ is weakly closed and weakly compact, since $\P(S)$ is weakly closed and weakly compact, and $\partial O$ is weakly closed. Therefore,
		\begin{equation*}
			m \coloneqq \min_{\mu\in \partial_{\P(S)} Q} \overline{V}(\mu)
		\end{equation*}
		exists, since $\overline{V}$ is weakly continuous. Notice that, since $\partial O \cap O = \emptyset$, it must be that $\partial_{\P(S)} Q \cap Q = \emptyset$, and therefore $\partial_{\P(S)}Q \cap P = \emptyset$. Hence, since $\overline{V}(\mu) > 0$ for all $\mu\in \P(S) \setminus P$, it must be that $\overline{V}(\mu) > 0$ for all $\mu\in\partial_{\P(S)} Q$ and thus $m > 0$.

		Now, let
		\begin{equation*}
			R = \{\mu\in Q : \overline{V}(\mu) \in (-\infty,m)\}.
		\end{equation*}
		Since $\overline{V}$ is weakly continuous and $(-\infty,m)$ is open, the preimage $\overline{V}^{-1}((-\infty),m)$ is weakly open, and hence $R = Q\cap \overline{V}^{-1}((-\infty,m)) = \P(S) \cap O \cap \overline{V}^{-1}((0,m))$ is relatively weakly open. Furthermore, since $P\subseteq Q$ and $P\subseteq V^{-1}((-\infty,m))$ as $\overline{V}(\mu) = 0$ for all $\mu\in P$, it holds that $P\subseteq R \subseteq \P(S)$. Let $\mu\colon [0,\infty) \to \P(S)$ be a solution to the EDM \eqref{eq: edm} with dynamics map $v$. Suppose that $\mu(0)\in R$. Then, since the Fr\'echet derivative of real-valued functions on $\R$ recovers the usual derivative, we have that
		\begin{equation*}
			\frac{d \overline{V}\circ \mu}{dt}(t) \epsilon = D(\overline{V}\circ \mu)(t)\epsilon = (D\overline{V}(\mu(t)) \circ D\mu(t)) \epsilon = D\overline{V}(\mu(t)) (\epsilon \dot{\mu}(t)) = \epsilon D\overline{V}(\mu(t)) v(\mu(t),F(\mu(t)))
		\end{equation*}
		for all $t \in [0,\infty)$ and all $\epsilon\in\R$, where we have used the chain rule for Fr\'echet differentiation, linearity of Fr\'echet derivatives, and the fact that $\mu$ is a solution to the EDM \eqref{eq: edm}. Hence,
		\begin{equation*}
			\frac{d \overline{V}\circ \mu}{dt}(t) = D\overline{V}(\mu(t)) v(\mu(t),F(\mu(t))) \le 0
		\end{equation*}
		for all $t\in[0,\infty)$. Since $\overline{V}$ is weakly continuous and $\mu$ is vaguely continuous and hence weakly continuous as $S$ is compact, we may apply the mean value theorem to find that $\overline{V}(\mu(t)) \le \overline{V}(\mu(0)) < m$ for all $t\in[0,\infty)$. Since $R\subseteq Q$, we conclude that $\mu(t) \in Q$ for all $t\in [0,\infty)$, so indeed $P$ is weakly Lyapunov stable under the dynamics map $v$.
	\end{proof}

	\begin{lemma}
		\label{lem: strict_lyapunov}
		Suppose that $S$ is compact. Consider a game $F\colon \P(S) \to C_0(S)$, let $v\colon \P(S) \times C_0(S) \to \M(S)$, and assume that \autoref{ass: exist_edm_solution} holds. Let $P\subseteq \P(S)$ be weakly closed. If there exists a strict global Lyapunov function for $P$ under the dynamics map $v$, then $P$ is globally weakly attracting under the dynamics map $v$.
	\end{lemma}

	\begin{proof}
		In this proof, we denote the complement of a subset $M \subseteq \M(S)$ by $M^c$.

		Suppose that there exists a strict global Lyapunov function $V\colon \P(S) \to \Rpl$ for $P$ under the dynamics map $v$, and let $\overline{V} \colon U\to \R$ be an appropriate extension as in \autoref{def: lyapunov_function}. Let $\mu_0\in\P(S)$ be an arbitrary initial state. Let $Q\subseteq \P(S)$ be relatively weakly open and contain $P$, and let $\mu\colon [0,\infty) \to \P(S)$ be the unique solution to the EDM \eqref{eq: edm} with initial state $\mu_0$ and dynamics map $v$. It suffices to show that there exists $T\in[0,\infty)$ such that
		\begin{equation}
			\mu(t)\in Q ~ \text{for all $t\in[T,\infty)$}.
			\label{eq: attracting_condition}
		\end{equation}
		Since $V$ is a global Lyapunov function, \autoref{lem: lyapunov} gives that $P$ is weakly Lyapunov stable under the dynamics map $v$, which implies that there exists a relatively weakly open set $R\subseteq \P(S)$ containing $P$ such that $\mu(t) \in Q$ for all $t\in [0,\infty)$ whenever $\mu(0)\in R$. By time-invariance of the EDM \eqref{eq: edm} and uniqueness of its solutions, if there exists $T\in[0,\infty)$ such that $\mu(T)\in R$, this implies that $\mu(t) \in Q$ for all $t\in [T,\infty)$. Thus, to prove \eqref{eq: attracting_condition}, it suffices to prove that there exists $T\in[0,\infty)$ such that $\mu(T)\in R$.

		For the sake of contradiction, suppose that $\mu(t) \notin R$ for all $t \in [0,\infty)$. Since $R$ is relatively weakly open, $R = \P(S) \cap O$ for some weakly open set $O\subseteq \M(S)$, and therefore $\P(S)\setminus R = \P(S) \cap (\P(S) \cap O)^c = \P(S) \cap (\P(S)^c \cup O^c) = \P(S) \cap O^c$ is weakly compact since $O^c$ is weakly closed and $\P(S)$ is weakly closed and weakly compact by \autoref{lem: P(S)_compact}. Hence,
		\begin{equation*}
			m \coloneqq \max_{\nu \in \P(S) \setminus R} D\overline{V}(\nu) v(\nu,F(\nu))
		\end{equation*}
		exists, since $\nu\mapsto D\overline{V}(\nu) v(\nu,F(\nu))$ is weakly continuous. Since $\P(S) \setminus R \subseteq \P(S) \setminus P$, it must hold that $m<0$ as $V$ is a strict global Lyapunov function. Furthermore, since $\mu(t) \in \P(S) \setminus R$ for all $t\in[0,\infty)$, it holds that
		\begin{equation*}
			\frac{d\overline{V}\circ \mu}{dt}(t) = D\overline{V}(\mu(t))v(\mu(t),F(\mu(t))) \le m
		\end{equation*}
		for all $t\in[0,\infty)$. Since $\overline{V}$ is weakly continuous and $\mu$ is vaguely continuous and hence weakly continuous as $S$ is compact, we may apply the mean value theorem to conclude that, for all $\tau\in (0,\infty)$, there exists $t\in (0,\tau)$ such that
		\begin{equation*}
			\frac{\overline{V}(\mu(\tau)) - \overline{V}(\mu(0))}{\tau} = \frac{d \overline{V}\circ \mu}{dt}(t) \le m,
		\end{equation*}
		and hence
		\begin{equation*}
			\overline{V}(\mu(\tau)) \le m \tau + \overline{V}(\mu(0))
		\end{equation*}
		for all $\tau\in (0,\infty)$. Since $m<0$, $m\tau + \overline{V}(\mu(0)) \to -\infty$ as $\tau \to \infty$, which implies that there exists $\tau\in (0,\infty)$ such that $\overline{V}(\mu(\tau)) < 0$. Since, for such $\tau$, it holds that $\mu(\tau)\in\P(S)\setminus R \subseteq \P(S) \setminus P$, this contradicts the property of the global Lyapunov function $V$ that $\overline{V}(\nu) > 0$ for all $\mu\in\P(S) \setminus P$. Therefore, the supposition that $\mu(t) \notin R$ for all $t\in[0,\infty)$ is false, and we conclude that indeed there exists $T\in [0,\infty)$ such that $\mu(T)\in R$, which completes the proof.
	\end{proof}
